# Supplementary material for: "I Want It That Way": Enabling Interactive Decision Support Using Large Language Models and Constraint Programming
Source: arXiv:2312.06908 source file (2024-10-01)
Supplement: Supplementary file 1 [file DISCERN-Supplementary.pdf]

# DISCERN Supplementary Materials

## Manager Task Instructions

### Task 1: Which day of the week should be a remote workday?

Options: Monday, Tuesday, Wednesday, Thursday, Friday

Your organization currently has a workplace policy for every worker to be fully on site. However, recent research has indicated that allowing one remote day a week may improve worker focus and productivity. Based on this, your organizational leaders have mandated that each manager confer with their team and decide on one day of a work week to work remotely by the end of the day. In making this decision, organizational leaders have advised that managers choose one day of the week after comparing how cross-team collaboration, productivity patterns, personal commitments, and team morale might be affected based on the choice of the day. They have also advised that the decision be equitable so that no one team member is disproportionately disadvantaged. However, they have left it up to your judgement to decide the extent to which these factors should affect the decision and to evaluate different days along these factors and make a final decision.

You know that most social events happen on Thursday and Friday so enforcing that your team works from home on those days could dampen team morale. Given your limited visibility into the team members' work routines, you have set up a meeting to invite input from different members to evaluate other factors for each day. For instance, for a given day you might ask each member whether they collaborate in-person with other teams on that day to evaluate the number of people whose cross-team collaborations would suffer if asked to work from home on that day.

Spend around 12-13 minutes list attributes that you think are relevant to evaluating the different options (Monday-Friday) and that might help you effectively solicit input from the team during the meeting. You may also use these tables to input your own assessments based on team input. You will have full control over which table/s you show to the team during the meeting.

### Task 2: Which hours of the day should be quiet hours?

Options: 9-11 am, 10-12 am, 11am-1pm, 1-3pm, 2-4pm, 3-5pm

Your organization, in an attempt to bolster productivity and promote a culture of focus, is considering the implementation of a daily "quiet hour" policy. This would involve a set 2-hour block of time each day during which employees are encouraged to concentrate on their work with minimal interruptions. Your organizational leaders have tasked each manager with discussing this with their teams and deciding on the quiet hours of a day by the end of the day. While deciding this, managers have been advised to consider the personal productivity rhythms, external collaboration patterns, disruption to existing routines. They have also stressed that this decision should be fair and should not unfairly disadvantage any team members. The actual weight of these factors and how they are assessed in the final decision, however, is left up to your judgement.

It's important to note that the timing of these quiet hours could potentially interfere with regular work habits, collaborative meetings, or even personal commitments. Moreover, it's a well-known fact in your organization that the after-lunch hours are usually more social and team bonding oriented, so declaring those as quiet hours might impact the team culture adversely. Since you don't have a complete understanding of everyone's daily work routines, you have decided to arrange a meeting to gain insight from the team to make a well-rounded decision. For example, you might ask each team member about their peak productivity hours or when they usually schedule their collaborative meetings.

Take about 12-13 minutes to list attributes that you believe are essential for evaluating different options (like morning hours, mid-day, afternoon, etc.) and that might assist you in effectively gathering input from your team during the meeting. You may also use these attributes to document your own evaluations based on team input. You have complete control over what you decide to present during the meeting.

## Team Member Instructions

### Alex Persona

Alex is a senior software engineer who's been with the company for five years. They live with their partner and their two young kids. They are highly motivated and productive and often take the lead on complex tasks.

*On remote workday:*

Alex prefers Monday to be the remote workday. Here’s what they have to say:

“I prefer to work remotely on Mondays as it's a day I designate for task outlining without interruptions. The day is usually devoid of cross-team interactions, so I leverage my post-weekend energy for coding. This remote start boosts my team's morale and provides a smooth transition from the weekend, allowing for personal commitments. These include managing Monday morning school routines for my kids, scheduled pediatric check-ups, and a personal morning jog. Furthermore, avoiding the chaotic Monday morning traffic and the lingering noise from neighbors' Sunday gatherings makes remote work on Monday the most logical and stress-free choice for me.”

Here’s a more detailed look at their thoughts:

Preferred Workload Distribution

- "Mondays are when I outline my tasks for the week, and being remote allows me to do so without interruptions."

Cross-Team Collaboration Patterns or Current Meeting Load

- "Most of my team meetings are later in the week, so Mondays are usually clear of cross-team interactions."

Energy Levels and Productivity Patterns

- "I'm super energized on Mondays after the weekend break. Being at home helps me channel that energy directly into coding without the distractions of office chatter."

Team Morale

- "Starting remotely on Monday helps me and my team get into the rhythm without the pressure of the office environment."

Week Division

- "Starting the week remotely on Monday sets a nice rhythm for me, giving me a jump start before the in-office days."

Extended Weekends

- "Working from home on Monday feels like a smooth transition from the weekend, especially after spending quality time with my kids."

Personal Commitments

- "After the weekend, Monday mornings can be hectic with getting the kids ready for school. Working remotely eases that morning rush."
- "I usually schedule routine pediatric check-ups for my kids on Monday mornings."
- "On Monday mornings, I like to take a quick jog around the park to kickstart my week. Being remote gives me that flexibility."
- "The Monday morning traffic after the weekend break is quite unpredictable, making the commute stressful."
- "My neighbors usually have gatherings that extend into Sunday nights. It's quieter during the day, so Mondays at home are ideal."

*On quiet hours:*

Alex prefers 9-11am to be quiet hours. Here's what they have to say:

“As a senior software engineer, I've observed that my peak productivity is between 9-11am. It's a window post the morning rush, right after I've settled my kids into their day, and right before any scheduled meetings or appointments. This block is crucial for diving deep into complex tasks, and it sets a positive, productive tone for the rest of the day. Hence, having 9-11am as quiet hours aligns perfectly with both my personal and professional rhythms, ensuring maximum efficiency and focus.”

Here's a more detailed look at their thoughts:

Preferred Workload Distribution:

- "I find 9-11am to be when I'm most alert and can handle complex coding challenges, so quiet hours during this time allow me to tackle them head-on without distractions."

Cross-Team Collaboration Patterns or Current Meeting Load:

- "I typically schedule my meetings for the afternoon, leaving 9-11am free. Having quiet hours then ensures I can focus on my tasks without interruptions."

Energy Levels and Productivity Patterns:

- "I'm most energetic and motivated during the late morning, so 9-11am quiet hours help me capitalize on this productive streak."

Team Morale:

- "Starting the day with a dedicated focus from 9-11am sets a positive tone for the rest of the day, boosting both my morale and the team's."

Day Division:

- "I like breaking my day into focused chunks, and 9-11am quiet hours allow me to complete a significant portion of work before lunch, setting a productive pace."

Use of Quiet Hours:

- "9-11am is when I dive into my deeper work tasks, utilizing the quiet hours for design and architecture decisions without being pulled into other commitments."

Personal Commitments:

- "With my kids settled in school by 9am, the 9-11am slot is ideal for quiet hours as I won't be disrupted by childcare responsibilities."
- "All my personal appointments are scheduled for the afternoon usually."
- "I've kept my personal hobbies and activities for the evening."
- "By 9am, the morning rush in our building subsides, and it becomes quieter, making 9-11am a conducive time for focused work without external distractions."

## Casey Persona

Casey is a mid-level developer who joined the company two years ago. They live alone and enjoy cycling and hiking during their free time.

### *On remote workday:*

Casey prefers Tuesday to be the remote workday. Here's what they have to say:

"As an mid-level developer, I find Tuesdays ideal for remote work. It allows me to dive into detailed coding without the distractions of Monday's rush. I also have a lighter meeting load on Tuesdays, making it easier to focus. Personally, the day serves as a mini-respite in the week. Plus, it gives me the flexibility to indulge in my early morning cycling rides and avoid the weekly roadblocks near my residence. All in all, having Tuesday as my remote day perfectly balances my professional commitments and personal passions."

Here's a more detailed look at their thoughts:

Preferred Workload Distribution:

- "Tuesdays are when I like to delve into detailed coding since the start-of-the-week rush is behind me."

Cross-Team Collaboration Patterns or Current Meeting Load:

- "My Tuesdays are relatively light on meetings, making it an optimal day for uninterrupted work."

Energy Levels and Productivity Patterns:

- "While I start the week energetically on Monday, by Tuesday I appreciate the change in environment to maintain my productivity."

Team Morale:

- "Working remotely on Tuesday offers a brief change, preventing the week from feeling too monotonous and lengthy."

Week Division:

- "Having Tuesday as a remote day gives me a slight breather after starting the week in-office."

Extended Weekends:

- "A remote Tuesday feels like a pause, a mini-weekend, allowing me to recharge before diving back into the rest of the week."

Personal Commitments:

- "I have scheduled my regular bike maintenance on Tuesdays to ensure I'm set for my weekend rides."
- "I like to go on early morning cycling rides on Tuesdays with others in this cycling club that I am a member of, so working from home afterward helps me save on commuting time."

*On quiet hours:*

Casey prefers 11am-1pm to be quiet hours. Here's what they have to say:

"Being a mid-level developer, my day usually starts with team meetings and emails. By 11am, I'm geared up to dive deep into my development tasks, making 11am-1pm the ideal quiet hours for me. This slot not only aligns with my peak energy levels but also acts as a

bridge between the morning and afternoon, optimizing my productivity. Living alone and having personal hobbies like cycling and hiking means I value this period of undisturbed work before I switch to relaxation or planning my next adventure."

Here's a more detailed look at their thoughts:

Preferred Workload Distribution:

- "By 11am, I've had a chance to go through my emails and prepare my to-do list for the day. 11am-1pm is the perfect window for me to dive deep into development without interruptions."

Cross-Team Collaboration Patterns or Current Meeting Load:

- "Early mornings are typically when we have our team stand-ups and briefings. By 11am, those are out of the way, allowing me to focus on my tasks without the risk of meetings disrupting my flow."

Energy Levels and Productivity Patterns:

- "I've noticed I hit a peak in my energy levels and motivation around mid-morning to early afternoon. Quiet hours from 11am-1pm would help me harness that energy for the most demanding tasks."

Team Morale:

- "Setting aside 11am-1pm for quiet hours gives me the motivation to push through complex tasks, knowing that I'll have a break afterward, which acts as a morale boost."

Day Division:

- "Having quiet hours from 11am-1pm offers a clean break. It allows for concentrated work before lunch and ensures I'm set up for a productive afternoon post-lunch."

Use of Quiet Hours:

- "I like to utilize the 11am-1pm window for in-depth coding sessions or even occasionally for some R&D on new development methodologies."

Personal Commitments:

- "Living alone means I often take the responsibility of managing home tasks. But by 11am, any morning chores are sorted, and I can immerse myself in work."

- "I usually reserve my early mornings for a cycling session. By the time I'm back and freshened up, it's about 11am, and I'm all set to tackle my workday."
- "My weekends often involve hiking, so during the weekdays, especially around 11am-1pm, I like to catch up on any hiking-related research or plan my next trip during breaks. It's easier when I know this slot is undisturbed."
- "I value my solitude living alone, and 11am-1pm is when the outside world seems to quieten down a bit, making it the ideal quiet hour for me."

## Charlie Persona

Charlie is a systems analyst who's been with the company for six years. They live with their partner and two children. They are highly respected for their skills and dedication.

### *On remote workday:*

Charlie prefers Friday to be the remote workday. Here's what they have to say:

"Fridays, for me, are a blend of reflection, consolidation, and family. Having spent a majority of the week collaborating and collecting data, this day provides the solitude I need to analyze and report on my findings. It's not just about work; being home gives me the chance to witness my children's growth, participate in family activities, and even take part in neighborhood events. The absence of a hectic commute and the tranquility of home makes it an ideal day to work remotely, gearing me up for a rejuvenating weekend."

Here's a more detailed look at their thoughts:

Preferred Workload Distribution:

- "By Friday, I've accumulated all the data I need for analysis. Working from home helps me consolidate my findings without distractions."

Cross-Team Collaboration Patterns or Current Meeting Load:

- "The beginning and middle of my week is packed with meetings. Friday is when I synthesize the information and draft my reports, and doing so remotely is ideal."

Energy Levels and Productivity Patterns:

- "After a demanding week, Friday remote work helps me preserve my energy and lets me channel it towards analytical tasks."

Team Morale:

- "Having a remote Friday serves as a perk that drives my motivation throughout the week. It's also a great way to show trust and encourage autonomy in our team."

Week Division:

- "By taking Friday as a remote day, I can tie up any loose ends and prepare for the coming week without the buzz of the office around."

Extended Weekends:

- "Working from home on Fridays provides a smoother transition into the weekend, giving me more quality time with my family."

Personal Commitments:

- "My children have extracurricular activities on Fridays. Being home allows me to be more involved and support them."
- "Given the dynamics of the week, my partner and I have our bi-weekly financial review on Fridays. Being at home helps us synchronize our schedules."
- "Fridays are when my children showcase what they've learned during the week, be it a school project or a new hobby. I cherish these moments, and working from home allows me to be present."
- "Traffic congestion on Fridays can be unpredictable. Choosing to work remotely alleviates the commute stress."
- "My neighborhood has community events on Fridays. While I enjoy them, they can be a bit loud, making remote work a more feasible option."

### *On quiet hours:*

Charlie prefers 10am-12pm to be quiet hours. Here's what they have to say:

"For me, 10am-12pm is a golden period. After the initial syncs and system checks, this window offers the perfect opportunity to dive deep into analysis and problem-solving. Not only is it in sync with my peak productivity, but it also aligns with a quieter environment at home, especially given the construction break next door and my partner engaging our children. Establishing quiet hours during this time ensures an undistracted environment, setting a positive tone for the rest of the day."

Here's a more detailed look at their thoughts:

Preferred Workload Distribution:

- "By 10am-12pm, I've reviewed the systems' updates and statuses. Quiet hours during this period would help me deep dive into any issues or anomalies."

Cross-Team Collaboration Patterns or Current Meeting Load:

- "Most of my team meetings and syncs are scheduled for the early morning or post-lunch. 10am-12pm offers a window without disruptions, making it ideal for quiet hours."

Energy Levels and Productivity Patterns:

- "After my morning routine and initial team syncs, 10am-12pm is when my concentration peaks. Quiet hours would complement this productivity window perfectly."

Team Morale:

- "Setting quiet hours at 10am-12pm allows the team to have a focused, productive start, setting a positive momentum for the rest of the day."

Day Division:

- "I like the idea of breaking the morning with 10am-12pm quiet hours. It allows for a clear distinction between preliminary checks and deep analysis."

Use of Quiet Hours:

- "For refining my technical skills and understanding intricate system updates, quiet hours from 10am-12pm are ideal."

Personal Commitments:

- "Afternoons are often dedicated to family commitments, especially with my two children. Morning quiet hours from 10am-12pm ensures I can focus on work without personal disruptions."
- "Late mornings are free from personal appointments. It's the perfect window before lunch to engage in concentrated work, making 10am-12pm ideal for quiet hours."
- "My partner often engages the children in activities during late mornings, ensuring fewer distractions at home. This makes 10am-12pm a conducive period for focused work."
- "The construction next door usually pauses for their break around 10am-12pm. This unexpected quiet complements the work quiet hours, allowing for undisturbed focus."

## Jordan Persona

Jordan is a junior software engineer who's just finished their first year at the company. They live with their parents and two siblings and have a keen interest in video gaming.

### *On remote workday:*

Jordan prefers Wednesday to be the remote workday. Here's what they have to say:

"As a junior software engineer, Wednesdays at home offer the perfect mid-week balance. I can delve into tasks with a fresh perspective, free from the beginning-of-the-week meeting loads. The change of environment from office to home keeps me motivated. Plus, it's convenient to balance family responsibilities, especially with a busy household and our combined online commitments. Additionally, my gaming sessions on Wednesday evenings are crucial, and working remotely ensures I'm all set for them without any rush. Overall, Wednesday as a remote day balances my budding professional journey and my personal passions seamlessly."

Here's a more detailed look at their thoughts:

Preferred Workload Distribution:

- "By Wednesday, I've usually got a grasp on the week's tasks. Working from home lets me tackle them without the usual office distractions."

Cross-Team Collaboration Patterns or Current Meeting Load:

- "The bulk of my team meetings are scheduled for the beginning of the week. Wednesdays are relatively free, making it easier to focus when remote."

Energy Levels and Productivity Patterns:

- "Come midweek, I sometimes need a change in environment to stay motivated and maintain my productivity levels."

Team Morale:

- "I feel that having a remote day in the middle of the week can act as a small break, recharging me for the rest of the week."

Week Division:

- "Working remotely on Wednesday splits my week perfectly. Two days in-office, a day remote, and then two more days in-office."

Extended Weekends:

- "Although Wednesday doesn't extend the weekend, it acts like a mid-week pause, giving me a chance to recharge."

Personal Commitments:

- "Living with my family means there's always something happening. Being at home on Wednesday helps me assist with some chores or family tasks."
- "On Wednesdays, I have scheduled sessions with a gaming mentor. Being remote makes it easier to fit this into my day."
- "Wednesdays are when my gaming group meets online for practice sessions in the evening. Working from home means I can join them without feeling rushed."
- "The midweek traffic can be unpredictable. It's convenient to skip the Wednesday commute."
- "With both my siblings and myself attending online classes or meetings, our home internet gets a heavy workout. By working remotely on Wednesday, I can manage my work tasks during non-peak home internet hours."

### *On quiet hours:*

Jordan prefers 8-10am to be quiet hours. Here's what they have to say:

"As a junior software engineer, my mornings from 8-10am are crucial. It's when my productivity is at its peak, and I can tackle intricate coding challenges head-on. The fact that team meetings are usually scheduled later gives me an uninterrupted window to focus. Living with my family means mornings can be bustling, but dedicating this time as quiet hours ensures I strike the right balance between familial obligations and professional growth. Plus, having a focused start allows me to indulge in my gaming passion later without any guilt."

Here's a more detailed look at their thoughts:

Preferred Workload Distribution:

- "First thing in the morning, around 8-10am, is when my mind is at its sharpest. I like to tackle complex coding challenges then, and quiet hours would significantly help."

Cross-Team Collaboration Patterns or Current Meeting Load:

- "Most team meetings and stand-ups are usually scheduled for later in the day, so I prefer my mornings, especially 8-10am, to be uninterrupted by meetings."

Energy Levels and Productivity Patterns:

- "I'm incredibly productive and energetic from 8-10am. That's when I'd like to dive deep into coding without disturbances."

Team Morale:

- "Starting the day with focused work from 8-10am gives me a sense of accomplishment early on, which sets a positive tone for the rest of the day."

Day Division:

- "I find that a concentrated work session from 8-10am helps me break the morning effectively, setting the pace for the rest of the day."

Use of Quiet Hours:

- "I'd use the quiet hours from 8-10am to refine my technical skills, diving deep into complex coding tasks or learning new software techniques."

Personal Commitments:

- "With my siblings getting ready for school and the house bustling, having my headphones on and focusing on work from 8-10am ensures I don't get distracted."
- "Since I live with my parents, the house gets quieter when everyone leaves, so I prefer to have a dedicated work focus from 8-10am before the day's chores begin."
- "I usually game late into the night. So, I prefer to start my day early with focused work from 8-10am, ensuring I maintain a balance between my profession and passion."
- "The mornings in our home can be a tad noisy with everyone starting their day. By dedicating 8-10am as quiet hours, I ensure I remain in my focused zone, even if the surrounding environment isn't ideal."

## Lee Persona

Lee is an experienced UI/UX designer who's been with the company for four years. They live with their spouse and cat, and they are deeply interested in art and design.

*On remote workday:*

Lee prefers Thursday to be the remote workday. Here's what they have to say:

"As a UI/UX designer, the ebb and flow of creativity play a crucial role in my job. Thursdays, for me, have always been a nexus of innovation and inspiration. Working remotely on this day allows me to marinate in my artistic inclinations, be it through fine-tuning designs based on feedback or indulging in personal art projects. With art classes and gallery visits often scheduled on this day, I find that the blend of professional design and personal artistry paints a holistic picture of fulfillment. Plus, spending some extra time with my cat is always a bonus."

Here's a more detailed look at their thoughts:

Preferred Workload Distribution:

- "By Thursday, I've collected most of the feedback on my designs, and remote work allows me to make refined adjustments in peace."

Cross-Team Collaboration Patterns or Current Meeting Load:

- "Early in the week, I collaborate extensively with developers and product teams. By Thursday, I prefer solo time to finalize my designs without interruptions."

Energy Levels and Productivity Patterns:

- "Thursdays have historically been my most creative days. Working from home fosters this creativity, letting me experiment with new design ideas."

Team Morale:

- "Taking Thursday off-site offers me a refreshing change of environment, recharging my creativity and ensuring I end the week strong."

Week Division:

- "Remote Thursdays offer a gentle transition to the weekend, letting me wrap up any lingering design tasks efficiently."

Extended Weekends:

- "While I enjoy office camaraderie, taking Thursday to work from home lets me slide into the weekend vibe a bit earlier, giving me a burst of energy."

Personal Commitments:

- "Thursdays are when I attend art classes in the evening. Working from home ensures I have ample time to transition between work and my art pursuits."
- "I've scheduled my monthly gallery visits for Thursdays. Being at home means I can quickly step out during a break without the hassle of a long commute."
- "My art studio at home beckons me during short breaks on Thursdays. It's invigorating to shift between design tasks and personal art projects."
- "With the local art community hosting events on Thursdays, being at home allows me to participate without worrying about the rush back to the office."
- "My cat tends to be more playful and needs attention on Thursdays. Working remotely ensures I can attend to her without it impacting my workflow."

*On quiet hours:*

Lee prefers 12-2pm to be quiet hours. Here's what they have to say:

"For me, 12pm-2pm represents a unique blend of personal and professional alignment. In this window, I am typically engaged in critical design assessments, sketching, and wireframing. With minimal collaboration meetings scheduled and an environment that is naturally quiet due to my cat's nap time and optimal natural lighting, these hours emerge as the best time for undistracted, focused work. Additionally, this period ensures a structured workflow leading up to their late lunch, making it the perfect quiet time."

Here's a more detailed look at their thoughts:

Preferred Workload Distribution:

- "12pm-2pm is when I often review design drafts and prototypes. Quiet hours would allow me to critically assess design details without interruption."

Cross-Team Collaboration Patterns or Current Meeting Load:

- "Most of my collaboration with developers and stakeholders happens in the mornings and late afternoons. The 12pm-2pm slot is relatively free, making it ideal for focused design work."

Energy Levels and Productivity Patterns:

- "Having a quiet period right around mid-day helps me channel my creative energy effectively before taking a short break."

Team Morale:

- "12pm-2pm quiet hours are a morale booster. It ensures everyone gets a dedicated time to focus amidst the hustle of the day, especially in the world of design."

Day Division:

- "Having 12pm-2pm as quiet hours gives a nice division to the day. It provides a structured work period before and after lunch."

Use of Quiet Hours:

- "I often use the 12pm-2pm window for sketching and wireframing. Having quiet hours during this time ensures that I can visualize user flows without disruptions."

Personal Commitments:

- "12pm-2pm is great as I usually take a late lunch after my spouse. Quiet hours ensure I utilize this time productively before breaking for a meal."
- "Our cat usually naps around this time, which means fewer distractions at home. It aligns well with work quiet hours, allowing for focused design work."
- "Incorporating elements of art into my designs requires deep concentration. The 12pm-2pm quiet hours align perfectly with this daily ritual, ensuring undivided attention."
- "The natural lighting in my workspace is optimal around mid-day, which is crucial for design work. Quiet hours from 12pm-2pm allow me to take full advantage of this."

## Morgan Persona

Morgan is a project manager who's been with the company for seven years. They live alone and enjoy reading and traveling in their free time.

### *On remote workday:*

Morgan prefers Tuesday to be the remote workday. Here’s what they have to say:

“As a project manager, my role demands a balance of team interaction and strategic planning. While Mondays are about syncing with the team, Tuesdays are my sanctuary for strategic thinking and mapping out the week. Working remotely then aids my focus, dovetailing beautifully with my love for reading and traveling. Whether it's catching up on a

new book, attending a travel expo, or simply enjoying the tranquillity of my home, a remote Tuesday ensures I get the best of both my professional and personal worlds.

Here’s a more detailed look at their thoughts:

Preferred Workload Distribution:

- "By Tuesday, I've gathered all the updates from my team and I need some quiet time to plan and allocate resources efficiently for the week ahead."

Cross-Team Collaboration Patterns or Current Meeting Load:

- "Mondays are swamped with team catch-ups and planning meetings. By Tuesday, I prefer to step back and work on the execution plan, making remote work ideal."

Energy Levels and Productivity Patterns:

- "After the rush of Monday, I find that Tuesday is when I am most focused and can effectively draft project timelines and strategies."

Team Morale:

- "Being away from the office on Tuesdays allows my team to work autonomously, building their confidence and decision-making skills."

Week Division:

- "Working remotely on Tuesday gives me an early break in the week, allowing a perfect blend of collaboration on Monday and focused work later."
- Extended Weekends:
- "Though I don't extend my weekends, having a remote Tuesday often allows me to take short trips and return on Monday evenings, making the most of my love for travel."

Personal Commitments:

- "I often join reading clubs or travel forums that meet on Tuesday evenings. Working from home ensures I can attend without the stress of commuting back from the office."
- "I schedule any personal appointments, like book launches or travel expos, for Tuesdays since I can manage them easily around my work when remote."
- "The quiet solitude of my home on a Tuesday is perfect for indulging in some reading during breaks."

- "Being at home on Tuesdays allows me the flexibility to receive any deliveries or handle any home maintenance without interrupting my work."
- "Living alone means I cherish the serene environment at home. Tuesdays are especially peaceful in my neighborhood, ensuring I can work with minimal distractions."

*On quiet hours:*

Morgan prefers 2-4pm to be quiet hours. Here's what they have to say:

"For me as an experienced project manager, 2pm-4pm emerges as a pivotal time for strategic planning, timeline reviews, and updating project management tools. This period, post the morning meeting rush, allows meto utilize the natural afternoon calm both in their professional and personal environment. My preference for a short reading break post-lunch makes the transition back to work smoother with the onset of quiet hours. Overall, these hours support me in staying organized and ahead in their role, especially given my evening personal commitments."

Here's a more detailed look at their thoughts:

Preferred Workload Distribution:

- "As a project manager, 2pm-4pm is when I typically sit down to plan the next day's tasks and review ongoing project timelines. Quiet hours then would be invaluable."

Cross-Team Collaboration Patterns or Current Meeting Load:

- "Mornings are often filled with team meetings and updates, but post-lunch, especially between 2pm-4pm, is a relatively calmer period suitable for focused strategic planning."

Energy Levels and Productivity Patterns:

- "I often experience an afternoon lull. The quiet hours between 2pm-4pm can provide the structured focus I need to push through and maintain productivity."

Team Morale:

- "Ensuring 2pm-4pm as quiet hours can act as a mid-afternoon morale boost, helping the team regain energy and focus for the latter half of the day."

Day Division:

- "Setting 2pm-4pm as quiet hours offers a distinct separation in the day, allowing for deep work after the bustle of morning meetings."

Use of Quiet Hours:

- "2pm-4pm is when I typically review and update our project management tools. Having quiet hours during this period ensures accuracy and attention to detail."

Personal Commitments:

- "Living alone, the afternoon provides a peaceful atmosphere at home. Setting 2pm-4pm as quiet hours aligns well with this natural tranquility."
- "Often, I take a short break post-lunch to read. Returning to work around 2pm, the quiet hours assist in smoothly transitioning back into work mode."
- "My evenings are sometimes occupied with travel planning or other personal engagements. Ensuring focused work from 2pm-4pm helps me stay ahead."
- "My residential area tends to be quieter in the early afternoons, making 2pm-4pm an optimal window for undistracted work."

## Riley Persona

Riley is a highly skilled QA engineer who's been with the company for three years. They live with their partner and two dogs and love spending time in the park with their pets.

*On remote workday:*

Riley prefers Thursday to be the remote workday. Here's what they have to say:

"As a seasoned QA engineer, having Thursdays as my remote workday aligns perfectly with the rhythm of my work. It's a day when I finalize testing cycles, and the peace of my home environment ensures attention to detail. While the professional aspect benefits immensely, my personal life gets a boost too. Whether it's spending quality time with my dogs, attending their training sessions, or indulging in photography at the park, a remote Thursday bridges my professional commitments and personal passions seamlessly."

Here's a more detailed look at their thoughts:

Preferred Workload Distribution:

- "Thursdays are when I typically finalize my testing cycles. The quiet of my home space allows me to concentrate on detailed work."

Cross-Team Collaboration Patterns or Current Meeting Load:

- "By Thursday, I've often had my main collaboration meetings for the week. This day lets me focus on implementing feedback from those interactions without interruptions."

Energy Levels and Productivity Patterns:

- "Towards the end of the week, I find a change in environment boosts my energy. Working from home on Thursdays ensures I maintain high productivity."

Team Morale:

- "Being remote on Thursday gives me a chance to recharge, ensuring I'm upbeat and proactive for our team roundups on Fridays."

Week Division:

- "Having Thursday as a remote day offers a good rhythm. It's like a prelude to Friday, helping me tie up loose ends before the week's close."

Extended Weekends:

- "Working remotely on Thursday provides a gentle transition into the weekend. It feels like easing into my personal time without a jarring switch."

Personal Commitments:

- "My partner and I have a routine of taking our dogs for longer park outings on Thursdays. Being home makes this much more manageable."
- "I've enrolled in a Thursday afternoon training class for one of our dogs. Being at home makes it easier to attend without a rush."
- "I've taken up photography as a hobby, and early Thursday evenings offer the best light for capturing the park's essence. Working from home lets me make the most of this."
- "The Thursday evening rush hour can be quite chaotic. Being remote ensures I avoid that completely."
- "Our neighborhood sometimes has community events on Thursday evenings. Working from home ensures I'm available without feeling stressed about commuting back in time."

*On quiet hours:*

Riley prefers 4-6pm to be quiet hours. Here's what they have to say:

"For me, 4pm-6pm stands out as a vital window that intersects both professional diligence and personal well-being. Professionally, this period is optimal for detailed analysis, report preparations, and test design. Meanwhile, on a personal front, it aligns with the time my partner takes the dogs out, ensuring a serene home environment. Moreover, wrapping up by 6pm ensures that I can then engage in rejuvenating walks in the park with my beloved pets, striking a harmonious work-life balance."

Here's a more detailed look at their thoughts:

Preferred Workload Distribution:

- "Late afternoons, specifically 4pm-6pm, are when I meticulously go over test results and log defects. A quiet environment during this time ensures accuracy."

Cross-Team Collaboration Patterns or Current Meeting Load:

- "Most of my collaborative sessions with developers occur in the mornings and early afternoons. By 4pm-6pm, I prefer focused testing and result analysis without meetings."

Energy Levels and Productivity Patterns:

- "I've observed that my attention to detail peaks in the late afternoon, making 4pm-6pm an ideal window for deep, uninterrupted QA work."

Team Morale:

- "A quiet period from 4pm-6pm helps our team wind down the day efficiently, ensuring that any detected issues can be addressed first thing the next morning."

Day Division:

- "With mornings typically reserved for test executions, 4pm-6pm provides a structured time to review results and prepare reports."

Use of Quiet Hours:

- "4pm-6pm is the time I often reserve for designing new test cases or refining existing ones. Quiet hours during this period allow for focused design thinking."

Personal Commitments:

- "Late afternoons are when my partner usually takes our dogs to the park, ensuring minimal distractions at home during my quiet hours."
- "With evening walks with my dogs in mind, I aim to wrap up major tasks by 6pm. Quiet hours before that help me achieve this."
- "To ensure quality time in the park without rushing, I need a focused work environment from 4pm-6pm. This ensures tasks don’t spill over into personal time."
- "My neighborhood usually sees increased activity in the evenings, but 4pm-6pm is relatively quiet, aligning well with my preference for those hours."

## Taylor Persona

Taylor is a database engineer who's been with the company for two years. They live in a flatshare with three other people and play in a local band.

### *On remote workday:*

Taylor prefers Friday to be the remote workday. Here’s what they have to say:

“Being a database engineer requires both collaborative and focused phases of work. While the initial part of the week is often filled with team interactions, Fridays are my days to consolidate and refine. Working from home then not only enhances my productivity but also meshes well with my personal passions. Whether it's rehearsing with my band, attending music lessons, or managing the vibrant energy of my flatshare, a remote Friday ensures a harmonious blend of my professional and musical worlds.”

Here’s a more detailed look at their thoughts:

Preferred Workload Distribution:

- "By Friday, I've usually mapped out the database needs for the upcoming week. Working from home allows me to finalize these plans without disturbances."

Cross-Team Collaboration Patterns or Current Meeting Load:

- "Most of my collaboration meetings are earlier in the week. Fridays give me the uninterrupted time I need to wrap up and optimize databases."

Energy Levels and Productivity Patterns:

- "I find myself more reflective and strategic towards the end of the week. Working remotely on Fridays supports this introspective work mode."

Team Morale:

- "Working from home on Fridays means I can avoid the end-of-week office buzz and concentrate on my tasks. Plus, it gives me a head-start into the weekend vibes."

Week Division:

- "Having a remote Friday lets me wind down the workweek smoothly. It feels like a buffer day between professional commitments and personal activities."

Extended Weekends:

- "Fridays are when my band often has late-night gigs or rehearsals. Working from home ensures I'm rested and prepared without the commute stress."

Personal Commitments:

- "Our band usually practices on Friday afternoons. Being remote means I can join them without any delay."
- "I occasionally have music lessons on Fridays to hone my skills. Being home ensures I can attend them without feeling rushed."
- "Given that I play in a local band, I sometimes have promotional or networking events on Fridays. Being remote gives me flexibility in managing these."
- "Considering the bustling atmosphere in my flatshare towards the weekend, being home on Fridays allows me to coordinate shared spaces for both work and leisure."
- "Living with three others means our flat can get noisy, especially on Fridays when everyone's in a weekend mood. Having it as my remote workday means I can choose to work from a quiet café or library if needed."

*On quiet hours:*

Taylor prefers 3-5pm to be quiet hours. Here's what they have to say:

"For me as a passionate database engineer, the timeframe of 3pm-5pm is a convergence of professional dedication and personal interests. It's the period post my team interactions, optimal for running intensive operations, troubleshooting, and optimizing databases. Living in a flatshare, this time also coincides with the quietest hours at home, ensuring undisturbed work. Moreover, with band practices often in the evenings, these quiet hours ensure that I remain efficient, wrapping up in time to delve into their musical pursuits."

Here’s a more detailed look at their thoughts:

Preferred Workload Distribution:

- "Afternoons, especially 3pm-5pm, are when I usually run my most resource-intensive database operations. Quiet hours then ensure I can monitor these tasks without distractions."

Cross-Team Collaboration Patterns or Current Meeting Load:

- "Mornings are typically allocated for team check-ins and updates. By 3pm-5pm, I'm free from collaborative tasks and can dive deep into complex database challenges."

Energy Levels and Productivity Patterns:

- "I tend to feel most inspired and focused during the late afternoon, so 3pm-5pm is a perfect window for quiet hours that complement this natural rhythm."

Team Morale:

- "Having quiet hours from 3pm-5pm acts as a boost, allowing our team to power through the final hours of the workday with renewed focus."

Day Division:

- "3pm-5pm quiet hours provide a structured break from morning and early afternoon tasks, helping divide the day into clear productivity phases."

Use of Quiet Hours:

- "I often reserve 3pm-5pm for database optimization and troubleshooting. Quiet hours during this period are invaluable for such meticulous work."

Personal Commitments:

- "Given my flatshare situation, most of my flatmates aren't home during 3pm-5pm, making it a naturally quieter time at home."
- "My band usually practices in the evenings. Having focused work hours from 3pm-5pm ensures I wrap up efficiently and have time for my music."
- "As I need to review and sometimes learn new music sheets for my band, ensuring work is streamlined from 3pm-5pm gives me ample evening time for this."
- "The communal areas in our flatshare become busier post 5pm. Ensuring my major tasks are done by then through the help of quiet hours is immensely beneficial.
